# Supplementary material for: Assisting Clinical Decisions for Scarcely Available Treatment via Disentangled Latent Representation
Source: arXiv:2307.03315 source file (2023-07-06)
Supplement: Supplementary file 1 [file Appendix_ISARIC.pdf]

**Setting and Data Sources**

The data was extracted from the COVID-19 database of hospitalized patients with SARS-CoV-2 infection included in the International Severe Acute Respiratory and Emerging Infection Consortium (ISARIC) WHO Clinical Characterisation Protocol International cohort (ISARIC Clinical Characterisation Group, 2020). This database utilized the ISARIC/WHO Clinical Characterisation Protocol for Severe Emerging Infections to collect data spanning 788 partner institutions and networks, covering 1651 sites across 63 countries from 26 January 2020 to 20 September 2021. Based on our knowledge, this is the largest COVID-19 in-hospital international database in the world including standardized clinical data. The study information is available on the ISARIC website (https://isaric.tghn.org).

**Participants and Outcome**

We included all patients with COVID-19 if the patients were admitted to ICU for at least 24 hours. This analysis included those with laboratory-confirmed SARS-CoV-2 infection detected by reverse-transcriptase (RT)-PCR or clinically diagnosed with COVID-19 according to the sites' local diagnostic methods. ICU duration time of patients was computed by start date and end date of ICU stay. Transferred patients during ICU stay were excluded from the patient list. The treatment outcome is defined as positive if the patient has received ECMO treatment during the hospitalization, and the ECMO is directly related to COVID-19. The mortality outcome is defined as positive if the patient died during the hospitalization. Transferred patients with unknown mortality status were excluded from the study.

**Data and Data Processing**

Input data were extracted from static variables and time-series records. Static variables included patient-related characteristics that were available at admission, including patient demographics and patient medical history, and comorbidities. Time series records were variables captured at different times after admission, including medication, laboratory results, and physiological parameters.

For statistic data in DM, VS, IN and SA tables of the ISARIC database, we extracted demographic, psychological, and comorbidities information. Numerical encoding was performed on the categorical features. For treatments listed in IN table, we performed one-hot encoding for each subcategory of treatments. Features with similar variables were composited into one, such as RACE and ETHNICITY.

For time-series data in IN, VS, and LB tables of the ISARIC database, our interesting records are those with timestamps before ECMO initiation day for positive patients and during hospitalization for negative patients. This was implemented by comparing the date of performance and ECMO initiation day or admission/discharge day of patients. After filtering, we identified features with multiple reporting units. The units were standardized into standard units per feature. In all interesting records, we kept the maximum or the minimum value as the worst performance of each feature based on the domain knowledge of clinicians.

We identified BMI(Body Mass Index), CCI(Charlson Comorbidity Index,  MAP(Mean Arterial Pressure), and PF RATO as features with high influence over results. To compensate for the high missing rate, we calculated their values based on data available and clinicians' domain knowledge with the formulas below. BMI and CCI were static features, so they only needed to be calculated once. MAP and PF RATIO were both time-series features. We found all required values in the formula with the same timestamp and calculated all available values. After calculation, we fill the original data with new values and extracted the one with the worst performance.

| | |
|---|---|
| BMI | $\frac{KG}{m^2}$ |
| CCI | https://www.mdcalc.com/charlson-comorbidity-index-cci |
| MAP | Diastolic Blood Pressure+$\frac{1}{3}$(Systolic Blood Pressure-Diastolic Blood Pressure) |
| PF RATIO | $\frac{PO_2}{FIO_2}$ |

Features with missing rates > 90% were excluded. To avoid data leakage, features with a strong relationship to the outcome were also dropped. For example, the treatment named 'EXTRACORPOREAL MEMBRANE OXYGENATION' in IN table was dropped as it indicated ECMO usage. To achieve better performance, features with ambiguous meanings such as "OTHER (NOT SPECIFIED)", and"OTHER SIGNS (NOT SPECIFIED)" were also excluded.

**Table 1.** Characteristics of the cohort. Categorical variables represented as frequency (%). Continuous variables represented as median (25th percentile, 75th percentile).

| **Name** | **All = 118801** | **Pos = 1451** | **Neg = 117350** | $p$ **value** |
|---|---|---|---|---|
| **AGE** | 58.00 (47.00, 68.00) | 52.00 (43.00, 61.00) | 58.00 (47.00, 68.00) | <0.001 |
| **Weight** | 79.90 (67.00, 93.05) | 87.50 (75.00, 102.03) | 79.00 (66.00, 92.94) | <0.001 |
| **Male sex, n (%)** | 68021 (57.26) | 999 (68.85) | 67022 (57.11) | <0.001 |

| | | | | |
|---|---|---|---|---|
| **Caucasian, n (%)** | 15423 (12.98) | 295 (20.33) | 15128 (12.89) | <0.001 |
| **ARDS, n (%)** | 17476 (14.71) | 970 (66.85) | 16506 (14.07) | <0.001 |
| **PULMONARY EMBOLISM OR DVT , n (%)** | 185 (0.16) | 18 (1.24) | 167 (0.14) | <0.001 |
| **NEUROLOGICAL COMPLICATION, n (%)** | 785 (0.66) | 38 (2.62) | 747 (0.64) | <0.001 |
| **CHRONIC PULMONARY DISEASE (NOT ASTHMA), n (%)** | 4919 (4.14) | 88 (6.06) | 4831 (4.12) | 0.0037 |
| **HYPERTENSION, n (%)** | 41405 (34.85) | 417 (28.74) | 40988 (34.93) | 0.9008 |
| **OBESITY, n (%)** | 11316 (9.53) | 423 (29.15) | 10893 (9.28) | <0.001 |
| **SMOKING, n (%)** | 9025 (7.6) | 187 (12.89) | 8838 (7.53) | <0.001 |
| **ACUTE KIDNEY INJURY, n (%)** | 11770 (9.91) | 628 (43.28) | 11142 (9.49) | <0.001 |
| **CHRONIC CARDIAC DISEASE (NOT HYPERTENSION), n (%)** | 7192 (6.05) | 88 (6.06) | 7104 (6.05) | 0.4793 |
| **MALIGNANT NEOPLASM, n (%)** | 1782 (1.5) | 32 (2.21) | 1750 (1.49) | 0.0963 |
| **ASTHMA, n (%)** | 7550 (6.36) | 170 (11.72) | 7380 (6.29) | <0.001 |
| **CHRONIC KIDNEY DISEASE, n (%)** | 4882 (4.11) | 83 (5.72) | 4799 (4.09) | 0.0190 |
| **SHOCK, n (%)** | 1180 (0.99) | 29 (2.0) | 1151 (0.98) | <0.001 |
| **PULMONARY EMBOLISM, n (%)** | 1478 (1.24) | 89 (6.13) | 1389 (1.18) | <0.001 |
| **SEIZURES, n (%)** | 304 (0.26) | 6 (0.41) | 298 (0.25) | 0.4877 |
| **DEEP VEIN THROMBOSIS, n (%)** | 266 (0.22) | 32 (2.21) | 234 (0.2) | <0.001 |

| | | | | |
|---|---|---|---|---|
| **ANEMIA, n (%)** | 7927 (6.67) | 559 (38.53) | 7368 (6.28) | <0.001 |
| **DIABETES MELLITUS - TYPE 1, n (%)** | 1426 (1.2) | 38 (2.62) | 1388 (1.18) | 0.4249 |
| **ANOREXIA, n (%)** | 873 (0.73) | 54 (3.72) | 819 (0.7) | <0.001 |
| **DIABETES MELLITUS - TYPE 2, n (%)** | 7355 (6.19) | 240 (16.54) | 7115 (6.06) | 0.2494 |
| **HYPOGLYCAEMIA, n (%)** | 1028 (0.87) | 85 (5.86) | 943 (0.8) | <0.001 |
| **STROKE, n (%)** | 754 (0.63) | 88 (6.06) | 666 (0.57) | <0.001 |
| **DEMENTIA, n (%)** | 756 (0.64) | 16 (1.1) | 740 (0.63) | 0.2857 |
| **HYPERGLYCAEMIA, n (%)** | 6995 (5.89) | 420 (28.95) | 6575 (5.6) | <0.001 |
| **CHRONIC NEUROLOGICAL DISORDER, n (%)** | 2978 (2.51) | 48 (3.31) | 2930 (2.5) | <0.001 |
| **CONGESTIVE HEART FAILURE, n (%)** | 1182 (0.99) | 54 (3.72) | 1128 (0.96) | <0.001 |
| **RHEUMATOLOGICAL DISORDER, n (%)** | 3675 (3.09) | 48 (3.31) | 3627 (3.09) | <0.001 |
| **PLEURAL EFFUSION, n (%)** | 2588 (2.18) | 273 (18.81) | 2315 (1.97) | <0.001 |
| **MYOCARDIAL INFARCTION, n (%)** | 250 (0.21) | 19 (1.31) | 231 (0.2) | <0.001 |
| **PNEUMOTHORAX, n (%)** | 1539 (1.3) | 199 (13.71) | 1340 (1.14) | <0.001 |
| **GASTROINTESTINAL BLEEDING, n (%)** | 1283 (1.08) | 111 (7.65) | 1172 (1.0) | <0.001 |
| **CHRONIC HAEMATOLOGICAL DISEASE, n (%)** | 1486 (1.25) | 33 (2.27) | 1453 (1.24) | 0.2396 |
| **VIRAL PNEUMONIA, n (%)** | 24109 (20.29) | 964 (66.44) | 23145 (19.72) | <0.001 |
| **COAGULATION DISORDER, n (%)** | 2813 (2.37) | 250 (17.23) | 2563 (2.18) | <0.001 |

| | | | | |
|---|---|---|---|---|
| **PANCREATITIS, n (%)** | 278 (0.23) | 14 (0.96) | 264 (0.22) | 0.0385 |
| **CARDIAC ARREST, n (%)** | 3310 (2.79) | 202 (13.92) | 3108 (2.65) | <0.001 |
| **BACTERIAL PNEUMONIA, n (%)** | 7174 (6.04) | 485 (33.43) | 6689 (5.7) | <0.001 |
| **RHABDOMYOLYSIS, n (%)** | 459 (0.39) | 41 (2.83) | 418 (0.36) | <0.001 |
| **BACTERAEMIA, n (%)** | 3647 (3.07) | 328 (22.61) | 3319 (2.83) | <0.001 |
| **CARDIAC ISCHAEMIA, n (%)** | 877 (0.74) | 51 (3.51) | 826 (0.7) | <0.001 |
| **CARDIOMYOPATHY, n (%)** | 347 (0.29) | 20 (1.38) | 327 (0.28) | 0.0028 |
| **CARDIAC ARRHYTHMIA, n (%)** | 4957 (4.17) | 305 (21.02) | 4652 (3.96) | <0.001 |
| **MILD LIVER DISEASE, n (%)** | 848 (0.71) | 17 (1.17) | 831 (0.71) | 0.1912 |
| **MODERATE OR SEVERE LIVER DISEASE, n (%)** | 614 (0.52) | 16 (1.1) | 598 (0.51) | 0.8955 |
| **IMMUNOSUPPRESSION, n (%)** | 612 (0.52) | 12 (0.83) | 600 (0.51) | 0.1818 |
| **ENDOCARDITIS, n (%)** | 133 (0.11) | 6 (0.41) | 127 (0.11) | 0.4341 |
| **LIVER DYSFUNCTION, n (%)** | 4536 (3.82) | 249 (17.16) | 4287 (3.65) | <0.001 |
| **CRYPTOGENIC ORGANIZING PNEUMONIA (COP) , n (%)** | 252 (0.21) | 27 (1.86) | 225 (0.19) | <0.001 |
| **MENINGITIS/ENCEPHALITIS, n (%)** | 198 (0.17) | 8 (0.55) | 190 (0.16) | 0.4084 |
| **MYOCARDITIS/PERICARDITIS, n (%)** | 354 (0.3) | 27 (1.86) | 327 (0.28) | 0.0008 |
| **ENDOCARDITIS/MYOCARDITIS/PERICARDITIS, n (%)** | 198 (0.17) | 7 (0.48) | 191 (0.16) | 0.6203 |
| **CHRONIC PULMONARY DISEASE (NOT SPECIFIED), n (%)** | 736 (0.62) | 7 (0.48) | 729 (0.62) | 0.0604 |

| | | | | |
|---|---|---|---|---|
| **SOLID ORGAN TRANSPLANT, n (%)** | 222 (0.19) | 5 (0.34) | 217 (0.18) | 0.8200 |
