# Supplementary material for: Assisting Clinical Decisions for Scarcely Available Treatment via Disentangled Latent Representation
Source: arXiv:2307.03315 source file (2023-07-06)
Supplement: Supplementary file 2 [file Appendix_Local_Dataset.pdf]

### Setting and Data Sources

Data was extracted from our institutional database of all patients tested for COVID-19. The database utilizes Epic electronic health record (EHR) data spanning 15 hospitals in the local healthcare system over a 19-month period (March 3rd 2020 to October 1st 2021). Patients who received ECMO underwent detailed chart review to confirm that ECMO was directly related to COVID-19.

The institutional review board approved the study with a waiver of consent. The Transparent Reporting of a Multivariable Prediction Model for Individual Prognosis or Diagnosis (TRIPOD) guidelines were used for the reporting of this study.

### Participants and Outcome

We included all patients with positive COVID-19 test, if the patients were admitted to ICU for at least 24 hours, and physical conditions eligible for ECMO treatment. The ECMO assignment is defined as positive, only if the patient has received ECMO treatment during the hospitalization, and the ECMO is directly related to COVID-19.

### Data and Data Processing

Input data were extracted from static variables, and time series records. Static variables included patient-related characteristics that were available at admission, including patient demographics and patient medical history and acuity. Time series records were variables captured at different times after admission, including lab tests, flowsheets and medications. Detailed feature engineering process and codes were provided in supplemental material.

**Table 1.** Characteristics of the cohort. Categorical variables represented as frequency (%). Continuous variables represented as median (25th percentile, 75th percentile).

| Features | Total cohort (n= 6247) | 1st wave | | | 2nd wave | | |
|---|---|---|---|---|---|---|---|
| | | ECMO (n=67) | Non-ECMO (n=2251) | *p* value | ECMO patients (n=68) | Non-ECMO patients (n=3861) | *p* value |
| Age, years | 54 [26, 64] | 54 [44, 59] | 58 [45, 65] | 0.007 | 55 [43, 61] | 48 [13, 63] | 0.005 |
| Male sex, n (%) | 3550 (57) | 46 (69) | 1255 (56) | 0.049 | 45 (66) | 2204 (57) | 0.168 |
| Caucasian, n (%) | 3965 (64) | 38 (57) | 1348 (60) | <0.001 | 42 (62) | 2537 (66) | 0.637 |
| Height, cm | 168 [157, 178] | 170 [163, 180] | 170 [163, 178] | 0.287 | 175 [168, 183] | 165 [145, 176] | <0.001 |
| Weight, kg | 76 [56, 95] | 85 [79, 105] | 84 [67, 100] | 0.03 | 88 [77, 109) | 71 [44, 91) | <0.001 |

| | | | | | | | |
|---|---|---|---|---|---|---|---|
| BMI, kg/m2 | 26 [20, 32] | 30 [26, 35] | 28 [24, 34] | 0.019 | 29 [26, 34] | 25 [19, 31] | <0.001 |
| Tobacco use, n (%) | 1207 (19) | 5 (7) | 500 (22) | 0.001 | 5 (7) | 697 (18) | 0.003 |
| SOFA[$] | 9 [6, 13] | 12 [10, 13] | 11 [7, 14] | 0.001 | 9 [6, 12] | 12 [9, 14] | <0.001 |
| Lowest PF ratio[$] | 112 [66, 204] | 56 [48, 69] | 107 [65, 201] | <0.001 | 55 [50, 63] | 126 [71, 218] | <0.001 |
| Hospital mortality, n (%) | 1079 (17) | 32 (48) | 391 (17) | <0.001 | 26 (38) | 630 (16) | <0.001 |
| CCI | 4 [1, 7] | 2 [1, 4.5] | 4 [2, 8] | <0.001 | 3 [1, 4] | 3 [1, 7] | 0.077 |
| Chronic pulmonary disease, n (%) | 2305 (37) | 18 (27) | 899 (40) | 0.042 | 13 (19) | 1375 (36) | 0.007 |
| Diabetes, n (%) | 2994 (48) | 36 (54) | 1388 (62) | 0.983 | 30 (44) | 1540 (40) | 0.562 |
| Malignancy, n (%) | 1537 (25) | 6 (9) | 594 (26) | 0.002 | 10 (15) | 927 (24) | 0.101 |
| Renal disease, n (%) | 1369 (22) | 13 (19) | 568 (25) | 0.346 | 9 (13) | 779 (20) | 0.206 |
| Hospital lengths-of-stay, days | 8 [4, 18] | 24 [13, 42] | 8 [4, 17] | <0.001 | 38 [27, 53] | 8 [4, 18] | <0.001 |
| Mechanical ventilation, days[$] | 2 [0, 7] | 10 [2, 22] | 3 [1, 10] | <0.001 | 21 [6, 37) | 4 [1, 15] | <0.001 |
| CRRT, n (%) | 386 (6) | 16 (24) | 145 (6) | <0.001 | 14 (21) | 211 (5) | <0.001 |
| Neuromuscular blockade, n (%) | 631 (10) | 45 (67) | 188 (8) | <0.001 | 56 (83) | 342 (9) | <0.001 |
| Nitric Oxide/Iloprost, n (%) | 511 (8) | 41 (61) | 196 (9) | <0.001 | 45 (67) | 229 (6) | <0.001 |

| | | | | | | | |
|---|---|---|---|---|---|---|---|
| Dopa. <5mcg/kg/min, Dobu., Milrinone or Levosimendan, n (%)$ | 592 (10) | 15 (22) | 145 (6) | <0.001 | 11 (16) | 421 (11) | 0.198 |
| Dopa. 5-15mcg/kg/min, Epi/NorEpi <0.1mcg/kg/min, Vaso, Phenyl, n (%)$ | 3219 (52) | 67 (100) | 1138 (51) | <0.001 | 68 (100) | 1946 (49) | <0.001 |
| Dopa >15mcg/kg/min, Epi/NorEpi >0.1mcg/kg/min, n (%)$ | 2154 (35) | 63 (94) | 726 (32) | <0.001 | 65 (96) | 1300 (33) | <0.001 |

$ Prior to ECMO initiation for ECMO patients or prior to discharge for non-ECMO patients

Data presented as median and interquartile range unless otherwise specified.

BMI = body mass index, CCI = Charlson Comorbidity Index, SOFA = Sequential Organ Failure Assessment, ECMO = Extracorporeal membrane oxygenation, CRRT = continuous renal replacement therapy, NPPV = non-invasive positive pressure ventilation, Dopa = Dopamine, Dobu = dobutamine, Epi = epinephrine, NorEpi = norepinephrine, Vaso = vasopressin, Phenyl = phenylephrine
