# Supplementary material for: Assisting Clinical Decisions for Scarcely Available Treatment via Disentangled Latent Representation
Source: arXiv:2307.03315 source file (2023-07-06)
Supplement: Supplementary file 3 [file supplementary1.tex]

\input{table3}
\input{figures/fig3.tex}
\input{algorithm}
